# Supplementary material for: A Concurrency-Optimal List-Based Set
Source: arXiv:1502.01633 source file (2021-01-14)
Supplement: Supplementary file 1 [file appendix.tex]

%!TEX root = paper-p.tex
\begin{figure*}[!h]
\begin{center}
 \includegraphics[scale=0.25]{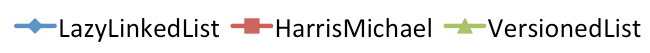}\\
 \includegraphics[scale=0.45]{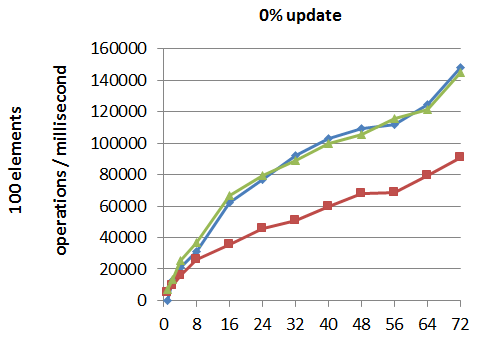}
 \includegraphics[scale=0.45]{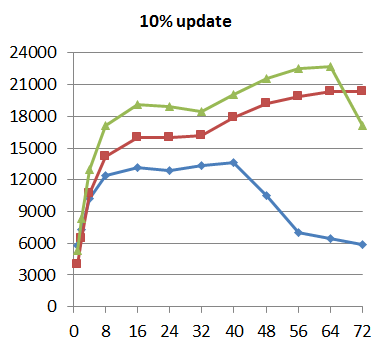}
 \includegraphics[scale=0.45]{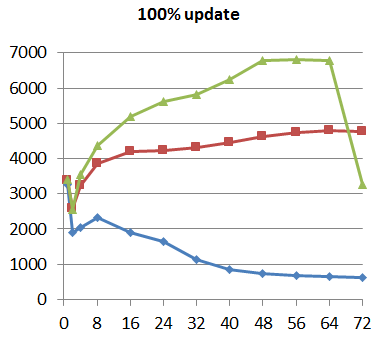}\\
 \includegraphics[scale=0.45]{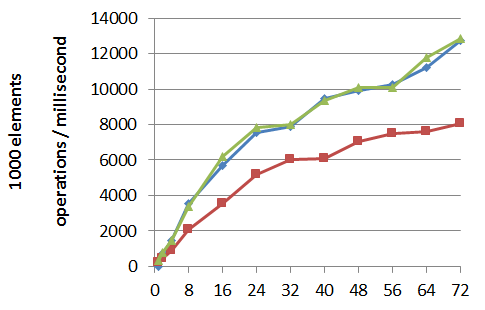}
 \includegraphics[scale=0.45]{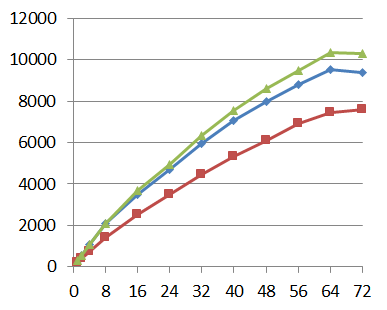}
 \includegraphics[scale=0.45]{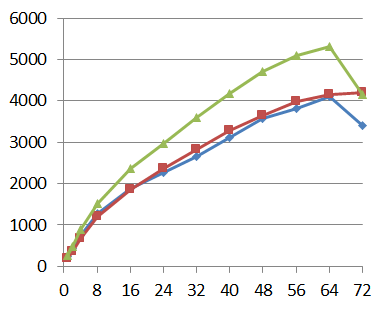}\\
 \includegraphics[scale=0.45]{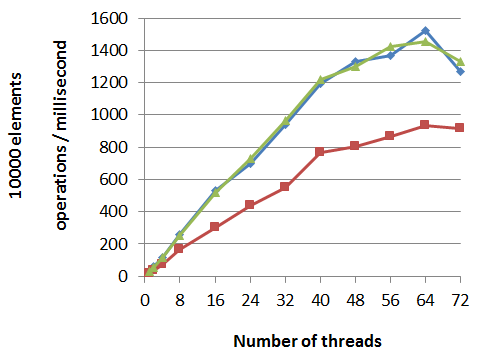}
 \includegraphics[scale=0.45]{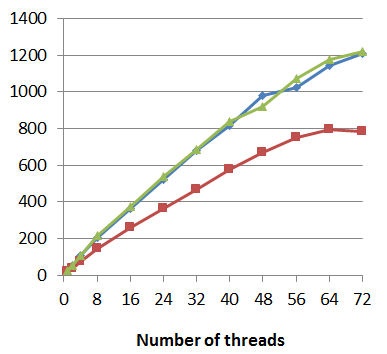}
 \includegraphics[scale=0.45]{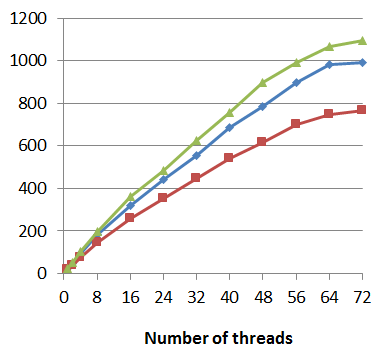}
\end{center}
%\vspace{-1.5em}
\caption{The performance results obtained on the x86 architecture\label{fig:x86}}
\end{figure*}

\begin{figure*}[!h]
\begin{center}
 \includegraphics[scale=0.25]{legends}\\
 \includegraphics[scale=0.45]{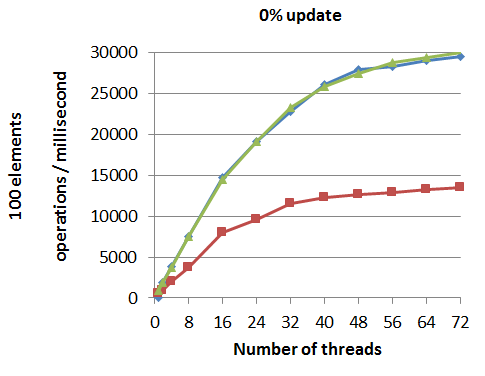}
 \includegraphics[scale=0.45]{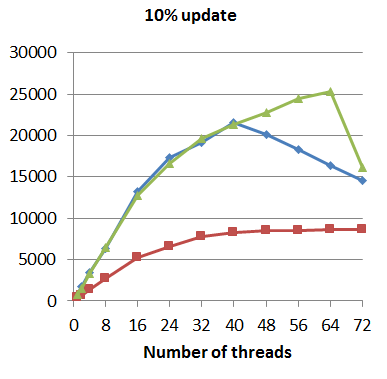}
 \includegraphics[scale=0.45]{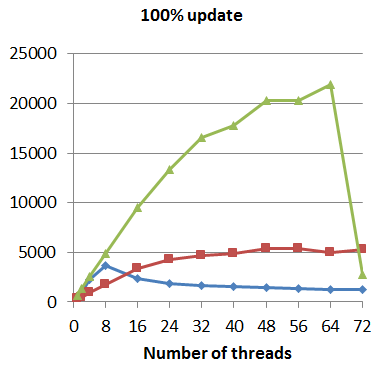}
\end{center}
%\vspace{-1.5em}
\caption{The performance results obtained on the SPARC architecture\label{fig:sparc}}
\end{figure*}
\section{Experimental evaluation of the versioned-list}
\label{app:exp}
We performed the experiment on a $4$ socket AMD Opteron 6378 $2.4$ GHz $16$-core ($64$-core in total) 
%The experiment was performed on a machine with AMD Opteron 6378 2.4 GHz 16 cores $\times$ 4 sockets for a total of 64 cores 
running Linux Fedora $18$ 
and on a Sun Niagara $2$ running SunOS $5.1$ with $8$ cores each running $8$ 
%HotSpot server 64-bit JVM 1.8-25 (SPARC and x86)
simultaneous multiple threads at $1.165$ GHz ($64$ hardware threads in total).
Both architectures run the 64-bit Java HotSpot server VM version 1.8 update 25.
%We also did the same experiment on a Sun Niagara 2 machine running SunOS 5.1 and Java 1.7 with 8 processors each running 8 simultaneous multiple threads at 1.165GHz for a total of 64 hardware threads.

Synchrobench initializes the data structure by filling it up to a predefined $\ms{size}$ 
with values chosen randomly from a $\ms{range} = \{1, 2, \ldots, 2\times\ms{size}\}$.
It spawns from $1$ to $72$ threads.  
Running for $10$ seconds,  each thread repeatedly chooses one of the three
operations with a fixed probability distribution 
function defined by the \emph{update ratio} 
and executes it  
with an argument picked uniformly at random from the $\ms{range}$. 
In the end, we sum up the number of operations completed from each thread and divide by the execution time 
of $10$ seconds to get the throughput rate. 

Note that the update ratio captures the amount of invoked $\lit{insert}$ and $\lit{remove}$, half of each typically fail. 
Hence out of 10\%
updates, only 5\% effectively modify the structure.
Here, the \emph{update ratio} defines the percentage of update operations,  where $\lit{insert}$ and $\lit{remove}$ 
are split in half for each: for example a $10\%$ update will result in $90\%$ $\lit{contains}$, $5\%$ $\lit{inserts}$ and 
$5\%$ $\lit{removes}$ (in average). 

%The rationale behind these workloads is that 
%(1) the performance is affected significantly by the size of the list and 
%(2) we want to keep the expected size of the list stable at runtime. 
The rationale behind the workload choice is to keep the size constant in expectation during the benchmark execution.
This is the case because both the $\lit{insert}$ and $\lit{remove}$ values are chosen from the \emph{range}
that is twice the initial size, which means both will have a $50\%$ chance to choose a value 
already in the list and same chance for the value to be absent. 
Note that the expected number of \emph{effective} $\lit{insert}$ (inserting a value absent in the list) 
and \emph{effective} $\lit{remove}$ (removing a value present in the list) is the half the update ratio. 

Our experiments are done for list sizes in $\{100, 1000, 10000\}$, 
update ratios in $\{0\%, 10\%, 100\%\}$ and number of concurrent
threads in $\{1, 2, 4, 8, 16, 24, \ldots, 72\}$. 
The results presented here are the average of $10$ runs of $10$ seconds
for each point in the parameter space.

Figures~\ref{fig:x86} and~\ref{fig:sparc} depict the number of operations per millisecond obtained on x86 and on SPARC, respectively.
We only report the results for a list size of $100$ on the SPARC architecture, 
since the curves on higher list sizes were similar for both architectures. 

The left column of both figures is the $\lit{contains}$-only workload, the right column is the update-only 
($\lit{insert}$ and $\lit{remove}$ only) workload, and the middle column is a more realistic workload with 90\% contains and 10\% updates. 
Note that the level of contention increases from bottom to top as the list size decreases 
(leading to a higher chance of concurrent threads accessing the same node) and 
left to right as the number of write operations increases. Also, since
each operation has 50\% chance to return $\false$, the
\emph{effective} updates are roughly half of the shown percentage. 

We also studied the contribution of  \emph{traversals} and
\emph{updates}  in the execution time used by $\lit{insert}$ and
$\lit{remove}$ in each algorithm.
The \emph{traversal} time is defined as the time between operation invocation and 
when it finds $prev$ and $curr$ where $prev.val < v \leq curr.val$ (including re-traversal time caused by abort and restart);
for our algorithm, we also include the time of $\lit{validate}$ function. 
The \emph{update} time is measured from just before locking to just after lock release; 
for Harris-Michael algorithm that does not use locks we simply
measured the time taken by the \emph{CAS} at the end of each update operation 
(excluding \emph{CAS}es that happen during list traversal). 
Table~\ref{tab:traversal} shows the relative execution time per operation per thread normalized by the lowest number 
among the data (shaded cell). 

\begin{table*}[!h]
\small
\begin{center}
\scalebox{0.8}[0.8]{

\begin{tabular}[t]{ | r |r| r | r | r | r | r | r | r | r | r | r | r | r |}

\hline
Operation & \multirow{2}{*}{Algorithm} & \multicolumn{12}{|c|}{Number of concurrent threads} \\
\cline{3-14}
segment &  &1& 2 & 4 & 8 & 16 & 24 & 32 & 40 & 48 & 56 & 64 & 72 \\
\hline
\multirow{3}{*}{Traversal} & Lazy linked list & 2.9 & 8.9 & 16.4 & 30.2 & 58.5 & 65.5 & 61.0 & 61.0 & 71.7 & 100.4 & 75.4 & 68.9 \\ 

& Harris-Michael & 5.2 & 9.9 & 15.9 & 29.2 & 59.0 & 91.4 & 127.9 & 153.3 & 177.1 & 203.2 & 228.9 & 252.8\\

& Versioned list & 3.7 & 7.2 & 12.3 & 22.8 & 42.3 & 61.5 & 79.5 & 89.2 & 96.0 & 109.6 & 122.2 & 202.9 \\

\hline
\multirow{3}{*}{Update} & Lazy linked list & 3.7 & 11.6 & 17.1 & 26.7 & 88.8 & 211.1 & 503.0 & 1019.5 & 1355.7 & 1814.6 & 2163.9 & 2634.2 \\ 

& Harris-Michael & \cellcolor[gray]{0.85} 1.0 & 3.8 & 4.8 & 5.4 & 6.4 & 7.0 & 8.3 & 9.4 & 10.2 & 11.1 & 12.9 & 13.7 \\

& Versioned list & 2.3 & 3.8 & 4.5 & 5.4 & 6.4 & 7.3 & 8.0 & 9.2 & 10.9 & 12.9 & 16.2 & 162.6 \\
\hline
\end{tabular}}
\vspace{-1.5em}
\caption{The relative time spent on list traversal and node update per operation on average using the benchmark with size 100 and update ratio 100\%\label{tab:traversal}}
\end{center}

\end{table*}
\newpage
\section{Versioned-lock implementation}
\label{app:vl}
\begin{algorithm*}[!h]
\caption{The CAS-based implementation for the versioned try-lock}
\label{alg:vlock}
  \begin{algorithmic}[1]
  	\begin{multicols}{2}
  	{\size
	
	\Part{Private field}{
		\State $\ms{lockValue}$, an integer that supports CAS
		\State Initially $\ms{lockValue} = 0$
	}\EndPart

	\Statex

% ------------- getVersion ---------------
	\Part{$\lit{getVersion}()$}{ \Comment {only return even value}
		\State {\bf return} $\ms{lockValue}$.read() \& $1111...1110$ 
	}\EndPart

	\Statex

% ------------- tryLockAtVersion ---------------
	\Part{$\lit{tryLockAtVersion}(ver)$}{ \Comment {assuming ver is even}
		\State {\bf return} $\ms{lockValue}$.CAS($ver$, $ver+1$) 
	}\EndPart

	\newpage

% ------------- lockAtCurrentVersion ---------------
	\Part{$\lit{lockAtCurrentVersion}()$}{ 
		\State $\ms{success} \gets \lit{false}$
		
		\While{($\neg \ms{success}$)} \Comment {spin until lock}
		\State $\ms{ver} \gets$ $\lit{getVersion()}$
		\State $\ms{success} \gets \ms{lockValue}$.$\lit{tryLockAtVersion}$($ver$)
		\EndWhile
	}\EndPart
	\Statex

% ------------- unlockAndIncrementVersion ---------------
	\Part{$\lit{unlockAndIncrementVersion}()$}{ \Comment{assumed locked (odd)}
		\State $\ms{val} \gets \ms{lockValue}$.read()
		\State $\ms{lockValue}$.CAS($val$, $val+1$) \Comment{could use atomicSet}
	}\EndPart

	}
	\end{multicols}
  \end{algorithmic}
\end{algorithm*}

\section{Linearizability and deadlock-freedom of the versioned-list}
\label{app:th1proof}
\setcounter{theorem}{0}
\begin{theorem}
\label{th:lr}
Versioned List is linearizable with respect to the $\ms{set}$ type.
\end{theorem}
\begin{proof}
Let $\alpha$ be a finite execution of Algorithm~\ref{alg:listver} and $<_\alpha$
denote the total-order on events in $\alpha$.
For the sake of the proof, we assume that $\alpha$ starts with an artificial
sequential execution of an insert operation $\pi_0$ that inserts $\ms{tail}$ and sets $\ms{head}.\ms{next}=\ms{tail}$. 
Let $H$ be the high-level history exported by $\alpha$.
%
%[[PK this does not appear in th main paper anymore
%Since \emph{linearizability} is a \emph{safety}
%property~\cite{Lyn96}, 
%it is sufficient for us to prove that every \emph{finite} high-level history $H$ is linearizable.
%]]

\vspace{0.8em}\noindent\textit{Completions.}
We obtain a completion $\tilde H$ of $H$ as follows.
The invocation of an incomplete $\lit{contains}$ operation is discarded.
The invocation of an incomplete $\pi=\lit{remove}$
operation that has not performed the write in Line~\ref{line:isdeleted} 
is discarded; otherwise, it is completed with response $\true$.
The invocation of an incomplete $\pi=\lit{insert}$
operation that has not performed the write in Line~\ref{line:inscommit} 
is discarded; otherwise, it is completed with response $\true$.

\vspace{0.8em}\noindent\textit{Linearization points.}
We obtain a sequential high-level history $\tilde S$ equivalent to $\tilde H$ by associating a linearization point $\ell_{\pi}$ 
with each operation $\pi$ as follows.
%
%\begin{itemize}
%\item 

For every $\pi=\lit{insert}(v)$ that returns $\true$ in $\tilde H$, $\ell_{\pi}$ is associated with 
%the last step of the \emph{tryCommit} (line~\ref{line:end-commit} of Algorithm~\ref{alg:elastic}) invoked in 
the write event in Line~\ref{line:inscommit} (rendering the node that
stores $v$ reachable from the \ms{head}); otherwise
$\ell_{\pi}$ is associated with the last $\lit{read}$ of a node's \emph{next} field performed by $\pi$ in $\alpha$. 

%\item
For every $\pi=\lit{remove}(v)$ that returns $\true$ in $\tilde H$, $\ell_{\pi}$ is associated with 
the write event in Line~\ref{line:isdeleted} (setting the
\ms{deleted} flag of a list's element); otherwise
$\ell_{\pi}$ is associated with the last $\lit{read}$ of a node's \emph{next} field performed by $\pi$ in $\alpha$. 

%\item
For $\pi=\lit{contains}(v)$ that returns $\true$, $\ell_{\pi}$
is associated with the last $\lit{read}$ performed by $\pi$ in which
$\pi$ finds the $\ms{deleted}$ field of a reachable node storing $v$ 
be $\false$ (Line~\ref{line:linr}).
%\item

For $\pi=\lit{contains}(v)$ that returns $\false$ in $H$, 
\begin{smallitemize}
\item
if $\pi$ reads $(X.value\neq v)$ in Line~\ref{line:linr}, where $X$ is the last node read by $\pi$ in $\alpha$,
$\ell_{\pi}$ is assigned to the read of the \emph{next} field of the node accessed by $\pi$ immediately before $X$
\item
if $\pi$ reads $(X.value = v)$ in Line~\ref{line:linr}, where $X$ is the last node read by $\pi$ in $\alpha$,
$\ell_{\pi}$ is defined as follows:
let $\pi_1$ be the $\lit{remove}$ operation that performs the last write
to $X.\ms{deleted}$ (Line~\ref{line:isdeleted}) prior to the read of $X.\ms{deleted}$ by $\pi$.
Then, $\ell_{\pi}$ is chosen to be the first event performed by $\pi_1$ immediately after the write to $X.\ms{deleted}$, but prior
the read of $X.\ms{deleted}$ by $\pi$. Otherwise if no such event of $\pi_1$ exists, then
$\ell_{\pi}$ is the read of $X.\ms{deleted}$ by $\pi$.
\end{smallitemize}
%
%\end{itemize}
%

Since linearization points are chosen within the intervals of 
operations performed in $\alpha$, for any two operations
$\pi_i$ and $\pi_j$ in ${\tilde H}$, if $\pi_i \rightarrow_{\tilde H}
\pi_j$, then $\pi_i \rightarrow_{\tilde S} \pi_j$.
We show that $\tilde S$ defined in Section~\ref{sec:vll} is consistent with the sequential specification of type \textit{set}.
When we refer to $\lit{read}(X)$, where
$X$ is a node, we mean the first read
of a node's field.

Let ${\tilde S}^k$ be the prefix of $\tilde S$ consisting of
the first $k$ complete operations. 
%(last event of ${\tilde S}^k$ is a response event).
%The state of the \emph{set} object at ${\tilde S}^0$ is $\emptyset$.
We associate each ${\tilde S}^k$ with a set $q^k$ of objects that were
successfully inserted and not subsequently successfully removed in ${\tilde S}^k$.
We show by induction on $k$ that the sequence of state transitions in
${\tilde S}^k$ is consistent with operations' responses in ${\tilde S}^k$ with respect to the \textit{set} type. 

%To prove that ${\tilde S}$ indeed consistent with \emph{set}, we
%proceed by induction on $k$. 
The base case $k=1$ is trivial: the \textit{tail} node containing
$+\infty$ is successfully inserted.
Suppose that ${\tilde S}^k$ is consistent with the \emph{set} type and
let $\pi_1$ with argument $v\in \mathbb{Z}$ and response $r_{\pi_{1}}$
be the last operation of ${\tilde S}^{k+1}$.  
We want to show that $(q^k,\pi_1,q^{k+1},r_{\pi_{1}})$ is consistent with the \textit{set} type. 
%We now prove that, upon the invocation of an operation $\pi_1$ with argument $v\in \mathbb{Z}$ applied at ${\tilde S}^k$ in state $q \in 2^{\mathbb{Z}}$,
%$(q,\pi_1,q',r_{\pi_{1}})$ is contained in the sequential
%specification of the \emph{set} type, where $q'$ is content of the
%\emph{set} object after ${\tilde S}^{k+1}$ defined in a natural way. We then say that ${\tilde S}^{k+1}$ satisfies $(q,\pi_1(v),q',r_{\pi_1})$.
%
%Let ${\tilde S}^k$ be the complete prefix of $\tilde S$ of length $k$.
%We proceed by induction on $k$.
%Let $\pi_1$ with argument $v\in \mathbb{Z}$ be the operation of the \emph{set} type applied at ${\tilde S}^k$ in state $q \in \mathbb{Z}$.
%

%\begin{enumerate}
\vspace{2mm}\noindent (1)
%\item[(1)]
Let $\pi_1=\lit{insert}(v)$ return $\true$ in ${\tilde S}^{k+1}$. 
We show below that each preceding $\pi_2=\lit{insert}(v)$ 
returning $\true$ is followed by $\lit{remove}(v)$ 
returning $\true$, such that
$\pi_2 \rightarrow_{{\tilde S}^{k+1}} \lit{remove}(v) \rightarrow_{{\tilde S}^{k+1}} \pi_1$.
Suppose the opposite. %by contradiction that such a $\pi_1$ and $\pi_2$ exist.
Observe that $\pi_1$ performs its penultimate $\lit{read}$ on a node $X$ 
that stores a value $v'<v$ and the last read is performed on a node that stores a value $v''>v$. 
%Clearly, $\pi_1$ also performs a $\lit{write}$ on $X$.
By construction of $\tilde S$, $\pi_1$ is linearized at the write on node $X$ in Line~\ref{line:inscommit}.
Observe that $\pi_2$ must also perform a $\lit{write}$ to the node $X$ 
(otherwise it is easy to see that one of $\pi_1$ or $\pi_2$ would return $\false$).
By assumption, the write to $X$ in shared-memory by $\pi_2$ in Line~\ref{line:inscommit} 
precedes the corresponding write to $X$ in
shared-memory by $\pi_1$. 
But $\pi_1$ can return $\true$ from the \emph{cas} performed in Line~\ref{line:inslock} only after 
$\pi_2$ releases the versioned lock on $X_1$ by performing the event in Line~\ref{line:relinsert}.
Thus, $\pi_1$ could not have returned $\true$---a contradiction.

Let $\pi_1=\lit{insert}(v)$ return $\false$ in ${\tilde S}^{k+1}$.
We show that there exists a preceding $\pi_2=\lit{insert}(v)$ returning 
$\true$ that is not followed by  $\pi_3=\lit{remove}(v)$ returning
$\true$, such that
$\pi_2 \rightarrow_{{\tilde S}^{k+1}} \pi_3 \rightarrow_{{\tilde S}^{k+1}} \pi_1$. 
Suppose that such a $\pi_2$ does not exist. Thus, $\pi_1$ must perform
its last $\lit{read}$ on a node $X$ that stores value $v''>v$, acquire the versioned lock on $X$ (Line~\ref{line:inslock})
and return $\true$---a contradiction to the assumption that $\pi_1$ returned $\false$.

It is easy to verify that the conjunction of the above two claims proves that 
$\forall q\in Q$; $\forall v\in \mathbb{Z}$, ${\tilde S}^{k+1}$ satisfies $(q,\lit{insert}(v),q \cup \{v\},(v \not\in q))$.

\vspace{2mm}\noindent (2)
%\item[(2)]
If $\pi_1=\lit{remove}(v)$, similar arguments as applied to $\lit{insert}(v)$ prove that 
$\forall q\in Q$; $\forall v\in \mathbb{Z}$, ${\tilde S}^{k+1}$ satisfies $(q,\lit{remove}(v),q \setminus \{v\},(v \in q))$.

\vspace{2mm}\noindent (3)
%\item[(3)]
Let $\pi_1=\lit{contains}(v)$ return $\true$ in ${\tilde S}^{k+1}$. 
We show that there exists $\pi_2=\lit{insert}(v)$ returning \emph{true} 
that is not followed by any $\lit{remove}(v)$ returning \emph{true}, such that
$\pi_2 \rightarrow_{{\tilde S}^{k+1}} \lit{remove}(v) \rightarrow_{{\tilde S}^{k+1}} \pi_1$.
Recall that $\pi_1$ is linearized at the last $\lit{read}$ of an node, say $X$, performed by $\pi$ when 
$\pi$ reads the $\ms{deleted}$ field
of $X$ to be $\false$ (Line~\ref{line:linr}). 
By the algorithm, 
%Lemma~\ref{lem:invar1}, 
there exists
$\pi_2=\lit{insert}(v)$ such that $\pi_2 \rightarrow_{{\tilde S}^{k+1}} \pi_1$ 
(let $\pi_2$ be the latest such operation).
Suppose that there exists a $\lit{remove}(v)$ that returns
\emph{true}, such that
$\pi_2 \rightarrow_{{\tilde S}^{k+1}} \lit{remove}(v) \rightarrow_{{\tilde S}^{k+1}} \pi_1$.
Thus, $\lit{remove}(v)$ performs the write event in Line~\ref{line:isdeleted} prior to the 
read of $X.\ms{deleted}$ by $\pi_1$. But then $\pi_1$ must read $X.\ms{deleted}$ to be $\true$
and return $\false$---a contradiction.

Now, let $\pi_1=\lit{contains}(v)$ return $\false$ in ${\tilde S}^{k+1}$. 
Thus, (1) there exists a $\pi_2=\lit{remove}(v)$ returning
\emph{true} that is not  
%$\lit{insert}(v) \rightarrow_{S} \lit{contains}(v)$ or 
followed by any $\lit{insert}(v)$ returning \emph{true},
such that 
$\pi_2 \rightarrow_{{\tilde S}^{k+1}} \lit{insert}(v) \rightarrow_{{\tilde S}^{k+1}} \pi_1$, or
(2) there does not exist any $\lit{insert}(v)$ returning $\true$ such that
$\lit{insert}(v) \rightarrow_{{\tilde S}^{k+1}} \pi_1$.
We consider two cases:
\begin{smallitemize}
\item 
Suppose that $\pi_1$ reads $(X.value \neq v)$ in Line~\ref{line:linr}, where $X$ is the last node read by $\pi_1$ in $\alpha$.
Thus, $\ell_{\pi_1}$ is assigned to the read of the \emph{next} field of the node, say $X'$ accessed by $\pi_1$ 
immediately before $X$.
Assume by contradiction that there exists
$\pi_2=\lit{insert}(v)$ that returns \emph{true} such that 
there does not exist any $\lit{remove}(v)$ that returns \emph{true}; 
$\pi_2 \rightarrow_{{\tilde S}^{k+1}} \lit{remove}(v) \rightarrow_{{\tilde S}^{k+1}} \lit{contains}(v)$.
But then $\pi_1$ must read $(X.value = v)$ in Line~\ref{line:linr} and return $\true$---contradiction.
\item
Suppose that $\pi_1$ reads $(X.value = v)$ and $X.\ms{deleted}$ to be $\true$ in Line~\ref{line:linr}.
Clearly, there exists a $\pi_2=\lit{remove}(v)$ that is concurrent to $\pi_1$ and returns $\true$ in ${\tilde H}$.
By the assignment of linearization points, $\ell_{\pi_1}$ is assigned to the first event performed
by $\pi_2$ immediately after the write to $X.\ms{deleted}$, but prior to the read of $X.\ms{deleted}$ by $\pi_1$, where $X$
is the last node read by $\pi_1$. 
We consider two cases:
(1) Suppose that some such event of $\pi_2$ exists.
We claim that there does not exist any $\pi_3=\lit{insert}(v)$ that returns $\true$ such that
$\pi_2 \rightarrow_{{\tilde S}^{k+1}} \pi_3 \rightarrow_{{\tilde S}^{k+1}} \pi_1$.
Any such $\pi_2$ must acquire the versioned lock on $X'$ (Line~\ref{line:inslock}), 
the node read by $\pi_1$ immediately prior to $X$. 
Since $\pi_1$ reads $(X.value = v)$ and $X.\ms{deleted}$ to be $\true$, $\pi_2$ must also acquire the versioned lock
on $X'$ (Line~\ref{line:remlock}). By our assumption, $\ell_{\pi_2} \rightarrow_{{\tilde S}^{k+1}} \ell_{\pi_3}$.
Thus, $\pi_3$ acquires the versioned lock on $X'$ only after $\pi_2$ releases it in Line~\ref{line:relremove}.
But we linearize $\pi_1$ prior to $\ell_{\pi_3}$ by choosing it to be the event performed by $\pi_2$
in Line~\ref{line:delcommit}---a contradiction to our assumption that $\ell_{\pi_3} <_{\alpha} \ell_{\pi_1}$.
(2)
Otherwise, if no such event of $\pi_2$ exists, $\ell_{\pi_1}$ is chosen as
the read of $X.\ms{deleted}$ by $\pi_1$. Since $\pi_2$ does not release the versioned lock on $X'$
prior to the read of $X.\ms{deleted}$ by $\pi_1$, there does not exist any $\lit{insert}(v)$ that returns $\true$
such that 
$ \lit{insert}(v) \rightarrow_{{\tilde S}^{k+1}} \pi_1$. Now, by the assignment of linearization points,
$\pi_2 \rightarrow_{{\tilde S}^{k+1}} \pi_1$.
\end{smallitemize}
%
%
%\end{enumerate}
%
Thus, inductively, the sequence of state transitions in ${\tilde S}$
satisfies the sequential specification of the \textit{set} type. 
\end{proof}
\begin{theorem}
\label{th:deadlock}
The versioned list provides deadlock-freedom.
\end{theorem}
\begin{proof}
Suppose that an update operation $\pi$ fails to return a matching response after taking infinitely many steps.
Intuitively, $\pi$ fails to do so because (1) it is returned $\bot$ from the call to $\lit{validate}$ in Line~\ref{line:insert-validate}
for $\lit{insert}$ (and resp. Line~\ref{line:delete-validate} for $\lit{remove}$), or (2)
it fails to acquire the lock on the $\ms{prev}$ node in Line~\ref{line:inslock} for $\lit{insert}$ 
(and resp. Line~\ref{line:remlock} for $\lit{remove}$),
or (3) it fails to acquire the lock on the $\ms{curr}$ node during Line~\ref{line:spinlock} by $\lit{remove}$.

In Case (1), there exists a concurrent $\lit{remove}$ operation that is executing the code
in its critical section and must eventually return the response $\true$.
In Case (2), if $\pi$ returns $\false$ from the call to $\ms{prev}.\lit{tryLockatVersion}$, then
some concurrent update operation has indeed succeeded to acquire the lock and enters its critical section
if its an $\lit{insert}$. Otherwise if this concurrent operation is a $\lit{remove}$, we are in Case (3)
i.e. $\lit{remove}$ does not return from the call to $\ms{curr}.\lit{lockAtCurrentVersion}$ in Line~\ref{line:spinlock}.
Thus, some other update operation has acquired the lock on the $\ms{curr}$ node of this $\lit{remove}$. Note that we can
iteratively extend this execution, but the last such process performing an update operation must eventually enter the critical
section and return a matching response.
\end{proof}
